# Supplementary material for: Differentiable Black-box and Gray-box Modeling of Nonlinear Audio Effects
Source: arXiv:2502.14405 source file (2025-02-20)
Supplement: Supplementary file 1 [file _appendix.tex]

\clearpage
\section{Appendix}
\label{sec:appendix}

% ===
\subsection{Results Compressor/Limiter}
\input{TABLES/appendix/test-loss_comp}

\input{TABLES/appendix/val-and-test-loss_comp_ampeg-optocomp}
\input{TABLES/appendix/val-and-test-loss_comp_flamma-analogcomp}
\input{TABLES/appendix/val-and-test-loss_comp_yuer-dynacomp}
\input{TABLES/appendix/val-and-test-loss_comp_ua-1176ln}

\input{TABLES/appendix/metrics_comp_ampeg-optocomp}
\input{TABLES/appendix/metrics_comp_flamma-analogcomp}
\input{TABLES/appendix/metrics_comp_yuer-dynacomp}
\input{TABLES/appendix/metrics_comp_ua-1176ln}

\clearpage

% ===
\subsection{Results Overdrive}
\input{TABLES/appendix/test-loss_od}

\input{TABLES/appendix/val-and-test-loss_od_fulltone-fulldrive}
\input{TABLES/appendix/val-and-test-loss_od_hb-greentint}
\input{TABLES/appendix/val-and-test-loss_od_ibanez-ts9}
\input{TABLES/appendix/val-and-test-loss_od_diy-klon-centaur}

\input{TABLES/appendix/metrics_od_fulltone-fulldrive}
\input{TABLES/appendix/metrics_od_hb-green-tint}
\input{TABLES/appendix/metrics_od_ibanez-ts9}
\input{TABLES/appendix/metrics_od_diy-klon-centaur}
\clearpage

% ===
\subsection{Results Distortion}
\input{TABLES/appendix/test-loss_dist}

\input{TABLES/appendix/val-and-test-loss_dist_eh-bigmuff}
\input{TABLES/appendix/val-and-test-loss_dist_hb-dropkick}
\input{TABLES/appendix/val-and-test-loss_dist_hb-plexicon}
\input{TABLES/appendix/val-and-test-loss_dist_hb-rodent}

\input{TABLES/appendix/metrics_dist_eh-bigmuff}
\input{TABLES/appendix/metrics_dist_hb-dropkick}
\input{TABLES/appendix/metrics_dist_hb-plexicon}
\input{TABLES/appendix/metrics_dist_hb-rodent}

\clearpage

% ===
\subsection{Results Fuzz}
\input{TABLES/appendix/test-loss_fuzz}

\input{TABLES/appendix/val-and-test-loss_fuzz_custom-dynamic-fuzz}
\input{TABLES/appendix/val-and-test-loss_fuzz_hb-fuzzy-logic}
\input{TABLES/appendix/val-and-test-loss_fuzz_hb-silly-fuzz}
\input{TABLES/appendix/val-and-test-loss_fuzz_arturia-636-preamp}

\input{TABLES/appendix/metrics_fuzz_custom-dynamic-fuzz}
\input{TABLES/appendix/metrics_fuzz_hb-fuzzy-logic}
\input{TABLES/appendix/metrics_fuzz_hb-silly-fuzz}
\input{TABLES/appendix/metrics_fuzz_arturia-636-preamp}

\clearpage
% ===
\subsection{Results Parametric Models}
\input{TABLES/appendix/val-and-test-loss_param_marshall-jvm410h}
\input{TABLES/appendix/val-and-test-loss_param_multidrive-ffuzz}

\input{TABLES/appendix/metrics_param_marshall-jvm410h}
\input{TABLES/appendix/metrics_param_multidrive-ffuzz}
